# Supplementary material for: Knowledge Guided Encoder-Decoder Framework: Integrating Multiple Physical Models for Agricultural Ecosystem Modeling
Source: arXiv:2505.06266 source file (2025-05-13)
Supplement: Supplementary file 1 [file Appendix.tex]

\section{Appendix}
\begin{table*}[]
\centering
\begin{tabular}{@{}cccccc@{}}
\toprule
Module                    & Feature       & \begin{tabular}[c]{@{}c@{}}DayCent \\ Encoder\end{tabular} & \begin{tabular}[c]{@{}c@{}}Decoder\\ (DayCent)\end{tabular} & \begin{tabular}[c]{@{}c@{}}Ecosys\\ Encoder\end{tabular} & \begin{tabular}[c]{@{}c@{}}Decoder\\ (Ecocsys)\end{tabular} \\ \midrule
\multirow{5}{*}{Carbon}   & Reco          & 0.836                                                        & -                                                             & 0.932                                                      & -                                                             \\
                          & GPP           & 0.896                                                        & 0.890                                                         & 0.920                                                      & 0.943                                                         \\
                          & CO2\_FLUX     & 0.886                                                        & 0.879                                                         & 0.919                                                      & 0.944                                                         \\
                          & Yield         & 0.957                                                        & 0.930                                                         & 0.830                                                      & 0.907                                                         \\
                          & Delta\_SOC    & 0.838                                                        & 0.746                                                         & 0.828                                                      & 0.785                                                         \\ \midrule
\multirow{5}{*}{Nitrogen} & N2O\_FLUX     & 0.306                                                        & 0.312                                                         & 0.753                                                      & 0.774                                                         \\
                          & NH4\_1        & 0.978                                                        & -                                                             & 0.79                                                       & -                                                             \\
                          & NO3\_1        & 0.958                                                        & -                                                             & 0.746                                                      & -                                                             \\
                          & NO3\_3        & 0.917                                                        & -                                                             & 0.811                                                      & -                                                             \\
                          & NO3\_5        & 0.862                                                        & -                                                             & 0.774                                                      & -                                                             \\ \midrule
\multirow{4}{*}{Water}    & WTR\_1        & 0.714                                                        & -                                                             & 0.810                                                      & -                                                             \\
                          & WTR\_3        & 0.819                                                        & -                                                             & 0.846                                                      & -                                                             \\
                          & WTR\_5        & 0.835                                                        & -                                                             & 0.815                                                      & -                                                             \\
                          & ET            & 0.894                                                        & 0.896                                                         & 0.852                                                      & 0.865                                                         \\ \midrule
\multirow{6}{*}{Thermal}  & TMAX\_SOIL\_1 & 0.938                                                        & -                                                             & 0.931                                                      & -                                                             \\
                          & TMIN\_SOIL\_1 & 0.933                                                        & -                                                             & 0.935                                                      & -                                                             \\
                          & TMAX\_SOIL\_3 & 0.981                                                        & -                                                             & 0.935                                                      & -                                                             \\
                          & TMIN\_SOIL\_3 & 0.980                                                        & -                                                             & 0.942                                                      & -                                                             \\
                          & TMAX\_SOIL\_5 & 0.976                                                        & -                                                             & 0.934                                                      & -                                                             \\
                          & TMIN\_SOIL\_5 & 0.976                                                        & -                                                             & 0.935                                                      & -                                                             \\ \bottomrule
\end{tabular}
\caption{Encoder performance}
\label{tab:surrogate-performance}
\end{table*}

\begin{figure*}[ht]
\centering
\includegraphics[width=0.85\textwidth]{figures/N2O (2).PNG}
\caption{Model Performance of N$_2$O Across Sites of Observation Data}
\label{fig:n2o_site}
\end{figure*}

\begin{figure*}[!htbp]
\centering
\includegraphics[width=0.98\textwidth]{figures/MS_2 (2).png}
\vspace{-.1in}
\caption{Comparison between predicted and ground truth weights for the four encoder modules: carbon, water, thermal, and nitrogen. Each subplot presents the weight variation of the Ecosys for the specific module being tested, while the weights for the other three modules remain constant across the four combinations.}
\label{fig:ms_eval_2}
\vspace{-.1in}
\end{figure*}

\subsubsection{Simulated dataset (Ecosys)} is derived from an advanced agroecosystem model Ecosys, constructed using detailed biophysical and biogeochemical rules~\cite{Grant2001,Zhou2021}. It encompasses a comprehensive set of input features related to weather, soil, and management practices. The input variables include:
\begin{itemize}
    \item \textbf{Weather:} Daily maximum and minimum air temperature (TMAX, TMIN, units are $^\circ$C), precipitation (PREC, mm day$^{-1}$), radiation (RADN), maximum and minimum humidity (HUMIDITY), and wind speed (WIND).
    \item \textbf{Soil:} Soil bulk density (TBKDS), sand content (TCSAND, g kg$^{-1}$), silt content (TCSILT, g kg$^{-1}$), soil pH (TPH, unitless), and soil organic carbon content (TSOC, g C kg$^{-1}$).
    \item \textbf{Management:} Fertilizer application rate (FERTZR\_N, g N m$^{-2}$), planting day of the year (PDOY, day), and plant type (PLANTT, 1 for corn and 0 for soybean).
\end{itemize}

The output features of Dataset Ecosys are categorized into four primary groups:
\begin{itemize}
    \item \textbf{Carbon:} Ecosystem respiration (Reco, g C m$^{-2}$ day$^{-1}$), net ecosystem exchange (NEE, g C m$^{-2}$ day$^{-1}$), gross primary productivity (GPP, g C m$^{-2}$ day$^{-1}$), crop yield (Yield, kg ha$^{-1}$ year$^{-1}$), change in soil organic carbon (\(\Delta\)SOC, g C m$^{-2}$ year$^{-1}$), and leaf area index (LAI, fraction).
    \item \textbf{Nitrogen:} Nitrous oxide flux (N$_2$O, g N m$^{-2}$ day$^{-1}$), ammonium concentration ([NH$_4^+$], g Mg$^{-1}$) at different soil layers (5 cm, 20 cm, 30 cm), and nitrate concentration ([NO$_3^-$], g Mg$^{-1}$) at similar depths.
    \item \textbf{Water:} Soil water content (SWC, m$^3$ m$^{-3}$) at different layers (5 cm, 20 cm, 30 cm) and evapotranspiration (ET, mm day$^{-1}$).
    \item \textbf{Thermal:} Daily maximum and minimum soil temperature (Tsoil\_max, Tsoil\_min, $^\circ$C) at different layers (5 cm, 20 cm, 30 cm).
\end{itemize}

\subsubsection{Simulated dataset (DayCent)} is derived from another biogeochemical model DayCent, which is currently used by the Environmental Protection Agency (EPA) and United States Department of Agriculture (USDA) for the U.S. national inventory of agricultural GHG emissions~\cite{Necpalova2015,DelGrosso2020}. This dataset shares the same input features as Dataset Ecosys but presents slight variations in its output features to reflect different measurement conditions and data availability. Specifically, this dataset includes the following output features:
\begin{itemize}
    \item \textbf{Carbon:} Similar to Dataset Ecosys, it covers Reco, NEE, GPP, yield, \(\Delta\)SOC, and LAI, though with slight definitional variations for some variables.
    \item \textbf{Nitrogen:} This dataset measures N$_2$O and provides ammonium concentrations ([NH$_4^+$]) only from the top 10 cm of soil, lacking measurements at deeper layers. Nitrate concentrations ([NO$_3^-$]) remain consistent across layers.
    \item \textbf{Water:} SWC and ET data are available with no negative values for ET, indicating atmospheric fluxes.
    \item \textbf{Thermal:} Soil temperatures are measured consistently at specified depths.
\end{itemize}
